# Supplementary material for: Synergistic signatures of group mechanisms in higher-order systems
Source: arXiv:2401.11588 source file (2024-10-24)
Supplement: Supplementary file 1 [file preamble_supp.tex]

\usepackage{amsmath}
\usepackage{amssymb}
% \usepackage{amsfonts}
\usepackage{amsthm}
\usepackage{chngcntr}
% \usepackage[ddmmyyyy]{datetime}
\usepackage{dcolumn}% Align table columns on decimal point
\usepackage{float}
\usepackage{graphicx} % Required for inserting images
\usepackage[colorlinks=true, allcolors=blue]{hyperref}
\usepackage{lipsum}
\usepackage{tabularray}
\bibliographystyle{apsrev4-2}
